# Supplementary material for: Ultrafast dynamics of neutral superexcited Oxygen: A direct measurement of the competition between autoionization and predissociation
Source: arXiv:1207.4740 source file (2012-10-15)
Supplement: Supplementary file 1 [file Supplementary_Material.pdf]

## Supplementary Information

To model the relaxation dynamics of superexcited Rydberg states and obtain the time-dependence of the ion-yield, we set up the rate equations characterizing the competition between autoionization and neutral dissociation. We invoke the core-ion model in which the Rydberg electron acts as a spectator to the dissociation dynamics of the system.

The time-dependent population of the $\nu = 0$ vibrational level in the $ns\sigma_g(c^4\Sigma_u^-)$ potential well of $O_2^{**}$ can be written as

$$P_o^{Ry}(t) = P_o e^{-t/\tau_a} e^{-t/\tau_d} \tag{1}$$

where $P_o$ is the initial population and the total rate of relaxation from the Rydberg well is a sum of the rates due to both autoionization, $1/\tau_a$, and neutral dissociation, $1/\tau_d$. The $\nu = 0$ population will predissociate into two prominent neutral dissociation limits, $nL1$ and $nL2$ (converging to the $L1$ and $L2$ ionic limits respectively) with rates $1/\tau_{d1}$ and $1/\tau_{d2}$. The predissociation rate can therefore be decomposed into

$$\frac{1}{\tau_d} = \frac{1}{\tau_{d1}} + \frac{1}{\tau_{d2}}, \tag{2}$$

For convenience, lets consider only the $L1$ channel - a clean channel which only measures counts from $\nu = 0$. We can express the rate equation for dissociation into the $nL1$ limit as

$$\frac{dP_o^{nL1}(t)}{dt} = \frac{1}{\tau_{d1}} P_o^{Ry}(t). \tag{3}$$

Using Eq. 1, the solution to this differential equation is given by

$$P_o^{nL1}(t) = P_o \left(\frac{\tau_d}{\tau_{d1}}\right) \frac{\tau_a}{\tau_d + \tau_a} (1 - e^{-t/\tau_a} e^{-t/\tau_d}), \tag{4}$$

Note that $\tau_d/\tau_{d1}$ represents the branching ratio into the $nL1$ limit.

In our experiment, the population in the Rydberg state will either decay due to the various relaxation mechanisms or a time-delayed IR pulse will excite the population into the ionic state. The population transferred to the ionic state is a reflection of the population remaining in the Rydberg potential well at any given time, or

$$P_o^{Ion}(t) = P_o^{Ry}(t) = P_o e^{-t/\tau_a} e^{-t/\tau_d}. \tag{5}$$

However, because the population in the $c^4\Sigma_u^-$ state is quasi-bound, it will also dissociate through various channels, giving rise to signals in both the $L1$ and $L2$ dissociation limits. To find the population in the $L1$ limit, we can multiply the time-dependent population by the branching ratio for the $L1$ channel to obtain

$$P_o^{L1}(t) = P_o \left(\frac{\tau_d}{\tau_{d1}}\right) e^{-t/\tau_a} e^{-t/\tau_d}. \tag{6}$$

In addition to the counts from the dissociation of $c^4\Sigma_u^-$, we will also have counts due to the IR ionization of any population in the $nL1$ limit. Assuming that the IR ionization cross-section does not vary significantly with the internuclear distance, the total ion yield in the $L1$ limit is given by

$$Y_{L1}(t) = P_o^{nL1}(t) + P_o^{L1}(t) = P_o \left(\frac{\tau_d}{\tau_{d1}}\right) \frac{\tau_d}{\tau_a + \tau_d} e^{-t/\tau_a} e^{-t/\tau_d} + P_o \left(\frac{\tau_d}{\tau_{d1}}\right) \frac{\tau_a}{\tau_a + \tau_d}. \tag{7}$$

Setting the branching ratio $\tau_d/\tau_{d1} = \alpha$, we get the equation 1 in the manuscript. The relative magnitudes for the coefficient of the exponential term and the dc baseline in Eq. 7 illustrate the competition between autoionization and neutral dissociation.

We can look at two different scenarios to see how the competition between different decay mechanisms manifests itself. In the first case, we consider $\tau_a << \tau_d$, or

$$Y_{L1}(t) = P_o\left(\frac{\tau_d}{\tau_{d1}}\right)e^{-t/\tau_a}. \tag{8}$$

When autoionization is the prominent decay mechanism, the ion yield will be lost to lower ionic states and data will exhibit a purely exponential decay and a zero dc baseline.

In the second limit, we consider $\tau_a >> \tau_d$, or

$$Y_{L1}(t) = P_o\left(\frac{\tau_d}{\tau_{d1}}\right). \tag{9}$$

When predissociation dominates, all of the ion counts are conserved since the population can either be ionized from the Rydberg potential well or the neutral dissociation limit and the data will exhibit no time delay dependence.

In an intermediate regime, the coefficient of the exponential decay term signifies the contribution of autoionization and the level of the dc baseline signifies the contribution of predissociation. It should be noted that the decay constant for the time dependence of the ion yield is always the sum of the autoionization and predissociation rates.

Under our experimental conditions, we excite two Rydberg state groups, both of which have identical neutral dissociation lifetimes but different autoionization lifetimes. As described in the manuscript, we define the quantity $r = (n^*_{5s,4d})^3/(n^*_{6s,5d})^3$ to be the scaling factor that gives the ratio of excitation probabilities and autoionization lifetimes between consecutive Rydberg states. We rewrite equation 7 as

$$Y_{L1}^{total}(t) = \alpha P_o\left[\frac{\tau_d}{\tau_a+\tau_d}e^{-t/\tau_d}e^{-t/\tau_a} + \frac{\tau_a}{\tau_a+\tau_d}\right] + \alpha r P_o\left[\frac{\tau_d}{(\tau_a/r)+\tau_d}e^{-t/\tau_d}e^{-t/(\tau_a/r)} + \frac{(\tau_a/r)}{(\tau_a/r)+\tau_d}\right]. \tag{10}$$

This equation is used in the data fitting procedure and the extraction of lifetimes.
